# Supplementary material for: LoRA-TTT: Low-Rank Test-Time Training for Vision-Language Models
Source: arXiv:2502.02069 source file (2025-02-04)
Supplement: Supplementary file 1 [file X_suppl.tex]

\setcounter{page}{1}

\section{Broader Impact}
\label{sec:impact}
Test-Time Training (TTT) for Vision-Language Models (VLMs) is crucial for enhancing their generalization ability and broadening their applicability to real-world AI applications.
This study introduces a novel method that achieves strong zero-shot generalization across diverse categories.
Our approach enables the development of systems that can adapt to various environments, ranging from memory-constrained edge devices to high-stakes applications, thereby making VLMs more versatile and practical in real-world scenarios.
We hope that Parameter-Efficient Fine-Tuning (\eg, LoRA) will play a pivotal role in TTT, inspiring future research aimed at improving the performance of foundation models.

\section{Limitations}
Our method has limitations that should be addressed in future work.
The MEM loss is primarily designed for image classification, making its adaptation to other tasks, such as object detection or segmentation, challenging.
In contrast, the MAE loss is task-agnostic, and extending it to such tasks is a promising direction.
Additionally, LoRA hyperparameters (e.g., $r$ and $\gamma$) require careful tuning as their optimal values depend on the target domain.
Developing a mechanism to dynamically adjust these parameters based on domain characteristics could improve adaptability and performance.

\begin{comment}
Our method has several limitations that should be addressed in future work.
\newline

\noindent\textbf{Architecture.}\hspace{5mm}
LoRA is primarily used for transformer-based architectures.
Similarly, the reconstruction approach based on MAE is also limited to transformer-based architectures, restricting its generalizability to other model types.
\newline

\noindent\textbf{Downstream task.}\hspace{5mm}
The MEM loss is primarily designed for image classification tasks, and its adaptation to other downstream tasks, such as object detection or segmentation, is not straightforward.
In contrast, the MAE loss is not specifically designed for any particular downstream task.
Thus, extending MAE loss to these tasks remains a promising direction for future work.
\newline

\noindent\textbf{Hyperparameter tuning.}\hspace{5mm}
Tuning LoRA hyperparameters (e.g., $r$ and $\gamma$) is crucial, as their optimal values vary depending on the target domain, as shown in \cref{fig:lora} of the main paper.
Developing a mechanism to dynamically adjust these hyperparameters based on domain characteristics could significantly enhance the method's adaptability and performance.
\end{comment}

\section{Experiments Details}

\subsection{Datasets}
The evaluation includes out-of-distribution testing on ImageNet and its four variants, as well as fine-grained classification assessments across categories derived from 10 different datasets.
The details of the datasets are provided in Table~\ref{tab:dataset}.

% I have confirmed that the test sizes match the actual data. (2024/8/30)
% I have confirmed that the number of classes matches the actual data. (2024/8/30)
\begin{table}[t]
\centering
\caption{\textbf{The details of the datasets used in the experiments.}}
\label{tab:dataset}
\begin{tabular}{lcc}
\toprule
\textbf{Dataset} & \textbf{\# Classes} & \textbf{Test set size} \\
\midrule
ImageNet \cite{deng2009imagenet} & 1,000 & 50,000 \\
ImageNet-A \citep{hendrycks2021natural} & 200 & 7,500 \\
ImageNetV2 \citep{recht2019imagenet} & 1,000 & 10,000 \\
ImageNet-R \citep{hendrycks2021many} & 200 & 30,000 \\
ImageNet-Sketch \citep{wang2019learning} & 1,000 & 50,889 \\
\midrule
\midrule
Flowers102 \citep{nilsback2008automated} & 102 & 2,463 \\
DTD \citep{cimpoi2014describing} & 47 & 1,692 \\
OxfordPets \citep{parkhi2012cats} & 37 & 3,669 \\
StanfordCars \citep{krause20133d} & 196 & 8,041 \\
UCF101 \citep{soomro2012ucf101} & 101 & 3,783 \\
Caltech101 \citep{li2022caltech} & 100 & 2,465 \\
Food101 \citep{bossard2014food} & 101 & 30,300 \\
SUN397 \citep{xiao2010sun} & 397 & 19,850 \\
FGVCAircraft \citep{maji2013fine} & 100 & 3,333 \\
EuroSAT \citep{helber2019eurosat} & 10 & 8,100 \\
\bottomrule
\end{tabular}
\end{table}

\subsection{Ensemble of text prompts}
The 80 hand-crafted prompts are listed in \cref{tab:ensemble}.

\begin{table*}[t]
    \centering
    \caption{The 80 hand-crafted text prompts.}
    \label{tab:ensemble}
    \begin{tabularx}{\textwidth}{X}
        \hline
        ``a bad photo of a \{ class \}'', ``a photo of many \{ class \}'', ``a sculpture of a \{ class \}'', ``a photo of the hard to see \{ class \}'', 
        ``a low resolution photo of the \{ class \}'', ``a rendering of a \{ class \}'', ``graffiti of a \{ class \}'', ``a bad photo of the \{ class \}'', 
        ``a cropped photo of the \{ class \}'', ``a tattoo of a \{ class \}'', ``the embroidered \{ class \}'', ``a photo of a hard to see \{ class \}'', 
        ``a bright photo of a \{ class \}'', ``a photo of a clean \{ class \}'', ``a photo of a dirty \{ class \}'', ``a dark photo of the \{ class \}'', 
        ``a drawing of a \{ class \}'', ``a photo of my \{ class \}'', ``the plastic \{ class \}'', ``a photo of the cool \{ class \}'', 
        ``a close-up photo of a \{ class \}'', ``a black and white photo of the \{ class \}'', ``a painting of the \{ class \}'', ``a painting of a \{ class \}'', 
        ``a pixelated photo of the \{ class \}'', ``a sculpture of the \{ class \}'', ``a bright photo of the \{ class \}'', ``a cropped photo of a \{ class \}'', 
        ``a plastic \{ class \}'', ``a photo of the dirty \{ class \}'', ``a jpeg corrupted photo of a \{ class \}'', ``a blurry photo of the \{ class \}'', 
        ``a photo of the \{ class \}'', ``a good photo of the \{ class \}'', ``a rendering of the \{ class \}'', ``a \{ class \} in a video game'', 
        ``a photo of one \{ class \}'', ``a doodle of a \{ class \}'', ``a close-up photo of the \{ class \}'', ``a photo of a \{ class \}'', 
        ``the origami \{ class \}'', ``the \{ class \} in a video game'', ``a sketch of a \{ class \}'', ``a doodle of the \{ class \}'', 
        ``a origami \{ class \}'', ``a low resolution photo of a \{ class \}'', ``the toy \{ class \}'', ``a rendition of the \{ class \}'', 
        ``a photo of the clean \{ class \}'', ``a photo of a large \{ class \}'', ``a rendition of a \{ class \}'', ``a photo of a nice \{ class \}'', 
        ``a photo of a weird \{ class \}'', ``a blurry photo of a \{ class \}'', ``a cartoon \{ class \}'', ``art of a \{ class \}'', 
        ``a sketch of the \{ class \}'', ``a embroidered \{ class \}'', ``a pixelated photo of a \{ class \}'', ``itap of the \{ class \}'', 
        ``a jpeg corrupted photo of the \{ class \}'', ``a good photo of a \{ class \}'', ``a plushie \{ class \}'', ``a photo of the nice \{ class \}'', 
        ``a photo of the small \{ class \}'', ``a photo of the weird \{ class \}'', ``the cartoon \{ class \}'', ``art of the \{ class \}'', 
        ``a drawing of the \{ class \}'', ``a photo of the large \{ class \}'', ``a black and white photo of a \{ class \}'', ``the plushie \{ class \}'', 
        ``a dark photo of a \{ class \}'', ``itap of a \{ class \}'', ``graffiti of the \{ class \}'', ``a toy \{ class \}'', ``itap of my \{ class \}'', 
        ``a photo of a cool \{ class \}'', ``a photo of a small \{ class \}'', ``a tattoo of the \{ class \}''. \\
        \hline
    \end{tabularx}
\end{table*}

\subsection{MAE loss variants}
In this section, we provide details about the variants of the MAE loss introduced in the main paper.
In addition to the MAE loss applied in \name, we explore the following approaches, as illustrated in \cref{fig:mae}.
The loss \( L_{\text{MAE}}^{\text{vis, enc}} \) calculates the mean squared error of unmasked visual tokens after image encoding.
The loss \( L_{\text{MAE}}^{\text{cls, dec}} \) reconstructs class tokens following the decoding process.
The loss \( L_{\text{MAE}}^{\text{pix, dec}} \) rearranges the visual tokens obtained after decoding back into image pixels, enabling pixel-level reconstruction.
This method of calculating \( L_{\text{MAE}}^{\text{pix, dec}} \)  is consistent with traditional TTT approaches based on MAE \cite{gandelsman2022test,wang2023test}.
These methodologies provide diverse perspectives on leveraging MAE loss for effective reconstruction.

\begin{figure*}[t]
\centering
\includegraphics[width=1.0\textwidth]{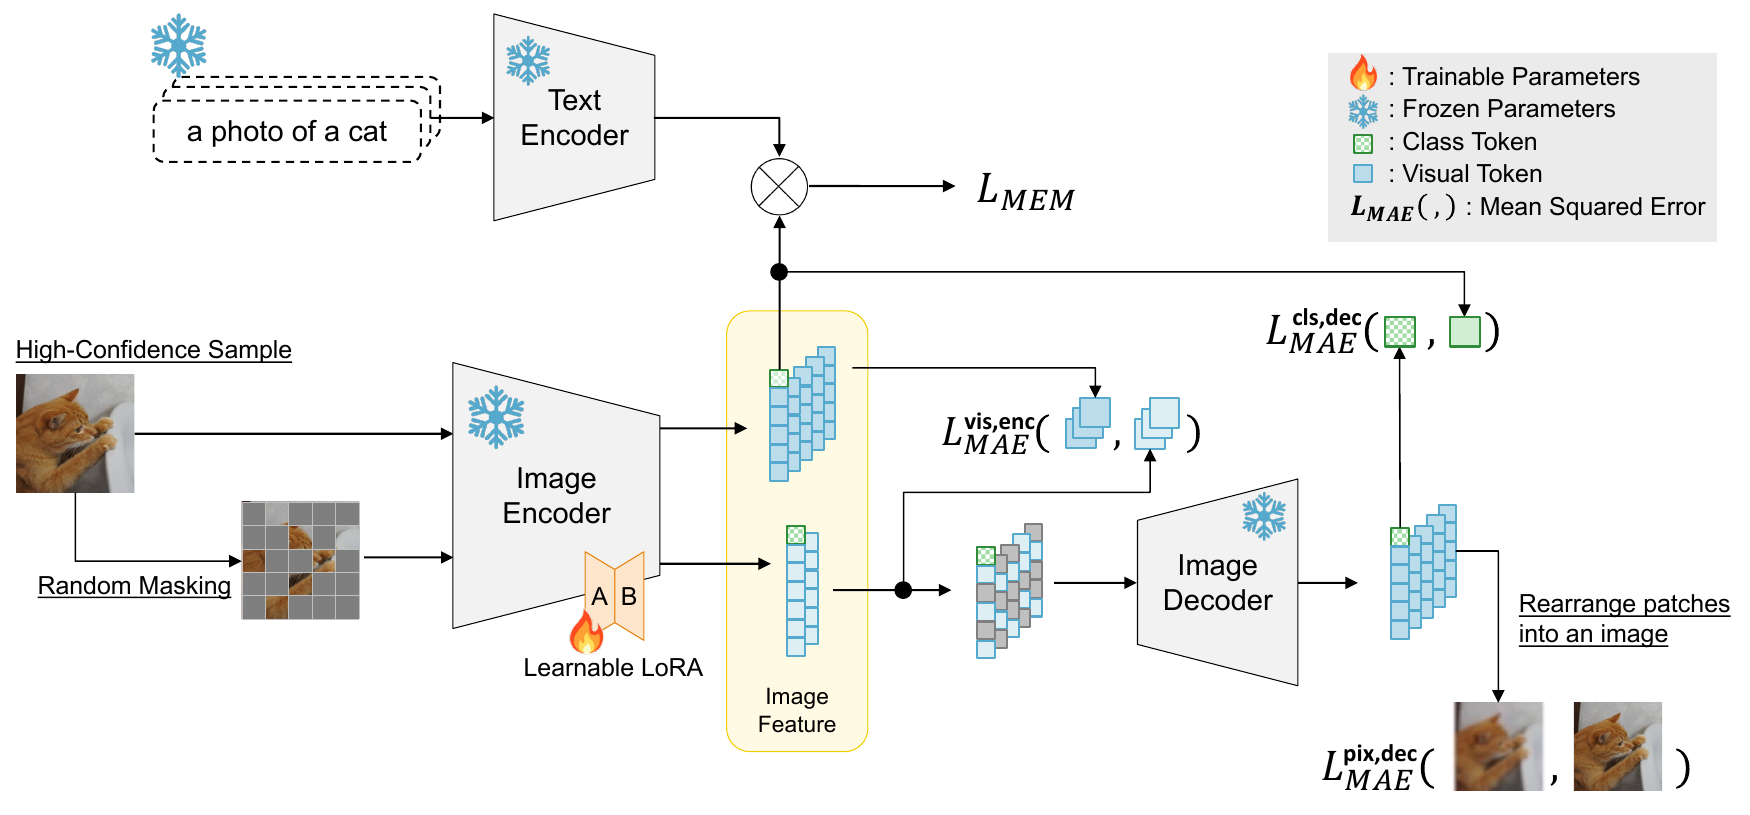}
\caption{\textbf{Variants of MAE Loss.}}
\label{fig:mae}
\end{figure*}

\subsection{Evaluation metric}
We use the Expected Calibration Error (ECE) \citep{naeini2015obtaining, yoon2024c} as a metric to evaluate the calibration performance of the model in image classification. 
ECE is calculated on a given evaluation dataset by dividing the model's outputs into equally sized bins based on prediction confidence and measuring the discrepancy between the predicted probabilities and the true probabilities within each bin.
A well-calibrated model exhibits a smaller gap between predicted confidence and actual accuracy, resulting in a lower ECE value.
The ECE is computed as follows:
\begin{equation}
\mathrm{ECE} = \sum_{k=1}^{K} \frac{|B_k|}{m} \left| \mathrm{acc}(B_k) - \mathrm{conf}(B_k) \right|,
\end{equation}
where \(K\) represents the number of bins, \(|B_k|\) denotes the number of samples in bin \(k\), \(\mathrm{acc}(B_k)\) is the average accuracy of the samples in bin \(k\), and \(\mathrm{conf}(B_k)\) represents the average prediction confidence of the samples in bin \(k\).
In our experiments, the number of bins is set to 20.

\section{Additional Experiments}

\begin{table*}[t]
\centering
\caption{Error analysis of top-1 accuracy in zero-shot image classification on the OOD benchmark.}
\label{tab:imagenets_error}
\begin{adjustbox}{width=0.9\textwidth}
\begin{tabular}{lccccccc}
\toprule
\rowcolor{gray!10} \textbf{Method} & \textbf{ImageNet} & \textbf{ImageNet-A} & \textbf{ImageNet-V2} & \textbf{ImageNet-R} & \textbf{ImageNet-Sketch} & \textbf{Average} & \textbf{OOD Avg.} \\
\midrule
CLIP-ViT-B/16 & 66.71 & 47.80 & 60.63 & 73.99 & 46.15 & 59.06 & 57.14 \\
\midrule
TPT \citep{shu2022test} & 69.02 ($\pm .14$) & 54.73 ($\pm .11$) & 63.70 ($\pm .09$) & 77.15 ($\pm .06$) & 47.99 ($\pm .04$) & 62.52 ($\pm .03$) & 60.89 ($\pm .04$) \\ 
\rowcolor{blue!10} \textbf{\namemem} (Ours) & 69.21 ($\pm .05$) & 60.57 ($\pm .16$) & 64.28 ($\pm .08$) & 77.53 ($\pm .09$) & 48.73 ($\pm .04$) & 64.06 ($\pm .02$) & 62.78 ($\pm .02$)\\

\rowcolor{blue!5} \textbf{\namemae} (Ours) & 66.27 ($\pm .11$) & 52.55 ($\pm .35$) & 60.87 ($\pm .19$) & 75.57 ($\pm .09$) & 47.01 ($\pm .08$) & 60.45 ($\pm .06$) & 59.00 ($\pm .08$) \\

\rowcolor{blue!15} \textbf{\name} (Ours) & 69.40 ($\pm .08$) & 60.52 ($\pm .19$) & 64.43 ($\pm .12$) & 77.84 ($\pm .03$) & 48.94 ($\pm .05$) & 64.23 ($\pm .01$) & 62.93 ($\pm .02$) \\
\bottomrule
\end{tabular}
\end{adjustbox}
\end{table*}

\begin{table*}[t]
\centering
\caption{Error analysis of top-1 accuracy in zero-shot image classification on the fine-grained benchmark.}
\label{tab:fg_error}
\begin{adjustbox}{width=\textwidth}
\begin{tabular}{lccccccccccc}
\toprule
\rowcolor{gray!10} \textbf{Method}  & \textbf{Flower102} & \textbf{DTD} & \textbf{Pets} & \textbf{Cars} & \textbf{UCF101} & \textbf{Caltech} & \textbf{Food101} & \textbf{SUN397} & \textbf{Aircraft} & \textbf{EuroSAT} & \textbf{FG Avg.} \\
\midrule
CLIP-ViT-B/16 & 67.40 & 44.39 & 88.25 & 65.51 & 65.24 & 93.31 & 83.64 & 62.56 & 23.91 & 42.22 & 63.64 \\
\midrule
TPT \citep{shu2022test} & 68.98 ($\pm .18$) & 45.92 ($\pm .33$) & 87.27 ($\pm .20$) & 67.02 ($\pm .14$) & 68.99 ($\pm .15$) & 93.55 ($\pm .22$) & 85.00 ($\pm .06$) & 65.11 ($\pm .08$) & 23.76 ($\pm .36$) & 43.44 ($\pm .08$) & 64.91 ($\pm .04$) \\ 

\rowcolor{blue!10}\textbf{\namemem} (Ours) & 67.60 ($\pm .33$) & 46.04 ($\pm .25$) & 87.11 ($\pm .19$) & 67.81 ($\pm .16$) & 68.38 ($\pm .07$) & 93.59 ($\pm .13$) & 84.83 ($\pm .13$) & 64.61 ($\pm .09$) & 25.68 ($\pm .12$) & 39.27 ($\pm .23$) & 64.49 ($\pm .08$)\\
\rowcolor{blue!5}\textbf{\namemae} (Ours) & 68.33 ($\pm .02$) & 45.21 ($\pm .07$) & 88.72 ($\pm .13$) & 66.94 ($\pm .02$) & 66.35 ($\pm .34$) & 93.71 ($\pm .02$) & 84.39 ($\pm .05$) & 63.63 ($\pm .12$) & 25.38 ($\pm .20$) & 44.52 ($\pm .15$) & 64.72 ($\pm .04$) \\

\rowcolor{blue!15}\textbf{\name} (Ours) & 67.88 ($\pm .22$) & 45.86 ($\pm .12$) & 87.63 ($\pm .06$) & 67.72 ($\pm .03$) & 68.38 ($\pm .12$) & 93.83 ($\pm .16$) & 84.99 ($\pm .05$) & 64.59 ($\pm .11$) & 25.92 ($\pm .39$) & 43.23 ($\pm .33$) & 65.00 ($\pm .06$)\\
\bottomrule
\end{tabular}
\end{adjustbox}
\end{table*}

\begin{table*}[t]
\centering
\caption{\textbf{Expected Calibration Error (ECE$\downarrow$)} of zero-shot image classification with TTA on the OOD benchmark. The best results, except for the baseline, are highlighted in \textbf{bold}.}
\label{tab:imagenets_calib}
\begin{adjustbox}{width=0.9\textwidth}
\begin{tabular}{lccccccc}
\toprule
\rowcolor{gray!10} \textbf{Method} & \textbf{ImageNet} & \textbf{ImageNet-A} & \textbf{ImageNet-V2} & \textbf{ImageNet-R} & \textbf{ImageNet-Sketch} & \textbf{Average} & \textbf{OOD Avg.} \\
\midrule
CLIP-ViT-B/16 & 1.93 & 8.37 & 2.51 & 3.53 & 4.79 & 4.23 & 4.80 \\
\midrule
TPT \citep{shu2022test} & 10.61 & 15.35 & 11.85 & 4.97 & 16.14 & 11.78 & 12.08 \\
C-TPT \citep{yoon2024c} & 3.11 & \textbf{6.40} & 4.64 & 2.80 & 7.69 & \textbf{4.93} & \textbf{5.38} \\
\midrule
\textbf{\namemem} (Ours) & 20.32 & 25.47 & 22.66 & 12.65 & 30.25 & 22.27 & 22.76  \\
\rowcolor{blue!5} \textbf{\namemae} (Ours) & \textbf{2.97} & 9.60 & \textbf{4.13} & \textbf{1.35} & \textbf{7.28} & 5.07 & 5.59  \\
\textbf{\name} (Ours) & 14.04 & 19.27 & 16.19 & 8.08 & 22.45 & 16.00 & 16.49 \\
\bottomrule
\end{tabular}
\end{adjustbox}
\end{table*}

\begin{table*}[t]
\centering
\caption{\textbf{Expected Calibration Error (ECE$\downarrow$)} of zero-shot image classification with TTA on the fine-grained benchmark. The best results, except for the baseline, are highlighted in \textbf{bold}.}
\label{tab:fg_calib}
\begin{adjustbox}{width=\textwidth}
\begin{tabular}{l|ccccccccccc}
\toprule
\rowcolor{gray!10} \textbf{Method} & \textbf{Flower102} & \textbf{DTD} & \textbf{Pets} & \textbf{Cars} & \textbf{UCF101} & \textbf{Caltech} & \textbf{Food101} & \textbf{SUN397} & \textbf{Aircraft} & \textbf{EuroSAT} & \textbf{Average} \\
\midrule
CLIP-ViT-B/16 & 3.21 & 8.23 & 4.41 & 4.45 & 2.93 & 5.12 & 2.03 & 2.24 & 5.50 & 7.16 & 4.53 \\
\midrule
TPT \citep{shu2022test} & 13.57 & 23.45 & 6.18 & 5.92 & 11.65 & 3.60 & 4.49 & 11.94 & 17.81 & 18.48 & 11.71 \\
C-TPT \citep{yoon2024c} & 5.24 & 13.77 & \textbf{1.56} & \textbf{1.56} & \textbf{2.30} & \textbf{3.27} & 3.31 & 5.02 & \textbf{4.41} & 12.47 & 5.29  \\
\midrule
\textbf{\namemem} (Ours) & 24.27 & 34.64 & 10.97 & 16.96 & 18.91 & 4.61 & 11.96 & 20.80 & 25.45 & 28.70 & 19.73  \\
\rowcolor{blue!5} \textbf{\namemae} (Ours) & \textbf{4.10} & \textbf{12.27} & 3.08 & 2.20 & 3.52 & 4.09 & \textbf{1.83} & \textbf{3.01} & 6.51 & \textbf{7.34} & \textbf{4.80} \\
\textbf{\name} (Ours) & 19.54 & 26.05 & 6.68 & 7.73 & 11.30 & 2.31 & 7.94 & 13.15 & 16.76 & 16.02 & 12.75 \\
\bottomrule
\end{tabular}
\end{adjustbox}
\end{table*}

\begin{table*}[t]
\centering
\caption{\textbf{Top-1 accuracy of zero-shot image classification on the OOD benchmark with the CLIP-ViT-L/14 baseline}. Performance improvements over the zero-shot CLIP-ViT-L/14 are indicated with an upward blue arrow {\textcolor{blue}{($\uparrow$blue)}} and a downward red arrow {\textcolor{red}{($\downarrow$red)}}.}
\label{tab:imagenets_vit_l}
\begin{adjustbox}{width=0.9\textwidth}
\begin{tabular}{lccccccc}
\toprule
\rowcolor{gray!10} \textbf{Method} & \textbf{ImageNet} & \textbf{ImageNet-A} & \textbf{ImageNet-V2} & \textbf{ImageNet-R} & \textbf{ImageNet-Sketch} & \textbf{Average} & \textbf{OOD Avg.} \\
\midrule
CLIP-ViT-L/14 & 73.45 & 68.77 & 67.75 & 85.41 & 57.82 & 70.64 & 69.94 \\
CLIP-ViT-L/14 + Ensemble & 75.53 & 70.75 & 69.70 & 87.85 & 59.60 & 72.69 & 71.97 \\
\midrule
\rowcolor{blue!10} \textbf{\namemem} (Ours) & 75.20\textsubscript{\textcolor{blue}{($\uparrow$1.75)}} & 73.73\textsubscript{\textcolor{blue}{($\uparrow$4.96)}} & 69.74\textsubscript{\textcolor{blue}{($\uparrow$1.99)}} & 87.69\textsubscript{\textcolor{blue}{($\uparrow$2.28)}} & 59.76\textsubscript{\textcolor{blue}{($\uparrow$1.94)}} & 73.22\textsubscript{\textcolor{blue}{($\uparrow$2.58)}} & 72.73\textsubscript{\textcolor{blue}{($\uparrow$2.79)}} \\
\rowcolor{blue!5} \textbf{\namemae} (Ours) & 73.88\textsubscript{\textcolor{blue}{($\uparrow$0.43)}} & 69.91\textsubscript{\textcolor{blue}{($\uparrow$1.13)}} & 67.98\textsubscript{\textcolor{blue}{($\uparrow$0.23)}} & 85.99\textsubscript{\textcolor{blue}{($\uparrow$0.58)}} & 58.30\textsubscript{\textcolor{blue}{($\uparrow$0.49)}} & 71.21\textsubscript{\textcolor{blue}{($\uparrow$0.57)}} & 70.55\textsubscript{\textcolor{blue}{($\uparrow$0.61)}} \\
\rowcolor{blue!15} \textbf{\name} (Ours) & 75.07\textsubscript{\textcolor{blue}{($\uparrow$1.61)}} & 72.56\textsubscript{\textcolor{blue}{($\uparrow$3.79)}} & 69.24\textsubscript{\textcolor{blue}{($\uparrow$1.49)}} & 87.27\textsubscript{\textcolor{blue}{($\uparrow$1.86)}} & 59.48\textsubscript{\textcolor{blue}{($\uparrow$1.67)}} & 72.72\textsubscript{\textcolor{blue}{($\uparrow$2.08)}} & 72.14\textsubscript{\textcolor{blue}{($\uparrow$2.20)}}  \\
\rowcolor{blue!10}\textbf{\name} + Ensemble (Ours) & 77.03\textsubscript{\textcolor{blue}{($\uparrow$3.57)}} & 75.63\textsubscript{\textcolor{blue}{($\uparrow$6.85)}} & 71.86\textsubscript{\textcolor{blue}{($\uparrow$4.11)}} & 89.73\textsubscript{\textcolor{blue}{($\uparrow$4.32)}} & 61.41\textsubscript{\textcolor{blue}{($\uparrow$3.59)}} & 75.13\textsubscript{\textcolor{blue}{($\uparrow$4.49)}} & 74.66\textsubscript{\textcolor{blue}{($\uparrow$4.72)}}  \\ 
\bottomrule
\end{tabular}
\end{adjustbox}
\end{table*}

\begin{table*}[t]
\centering
\caption{\textbf{Top-1 accuracy of zero-shot image classification on the fine-grained benchmark with the CLIP-ViT-L/14 baseline}. Performance improvements over the zero-shot CLIP-ViT-L/14 are indicated with an upward blue arrow {\textcolor{blue}{($\uparrow$blue)}} and a downward red arrow {\textcolor{red}{($\downarrow$red)}}.}
\label{tab:fg_vit_l}
\begin{adjustbox}{width=\textwidth}
\begin{tabular}{lccccccccccc}
\toprule
\rowcolor{gray!10} \textbf{Method}  & \textbf{Flower102} & \textbf{DTD} & \textbf{Pets} & \textbf{Cars} & \textbf{UCF101} & \textbf{Caltech} & \textbf{Food101} & \textbf{SUN397} & \textbf{Aircraft} & \textbf{EuroSAT} & \textbf{FG Avg.} \\
\midrule
CLIP-ViT-L/14 & 76.21 & 52.42 & 93.05 & 76.91 & 73.72 & 95.17 & 88.58 & 67.68 & 30.03 & 55.09 & 70.89 \\
CLIP-ViT-L/14 + Ensemble & 75.92 & 54.73 & 93.05 & 77.78 & 75.89 & 95.62 & 89.20 & 70.15 & 31.86 & 51.70 & 71.59 \\
\midrule
\rowcolor{blue!10}\textbf{\namemem} (Ours) & 76.45\textsubscript{\textcolor{blue}{($\uparrow$0.24)}} & 54.14\textsubscript{\textcolor{blue}{($\uparrow$1.71)}} & 93.81\textsubscript{\textcolor{blue}{($\uparrow$0.76)}} & 78.34\textsubscript{\textcolor{blue}{($\uparrow$1.43)}} & 75.23\textsubscript{\textcolor{blue}{($\uparrow$1.51)}} & 95.05\textsubscript{\textcolor{red}{($\downarrow$0.12)}} & 89.32\textsubscript{\textcolor{blue}{($\uparrow$0.74)}} & 68.97\textsubscript{\textcolor{blue}{($\uparrow$1.29)}} & 33.30\textsubscript{\textcolor{blue}{($\uparrow$3.27)}} & 52.32\textsubscript{\textcolor{red}{($\downarrow$2.77)}} & 71.69\textsubscript{\textcolor{blue}{($\uparrow$0.81)}} \\
\rowcolor{blue!5}\textbf{\namemae} (Ours) & 76.65\textsubscript{\textcolor{blue}{($\uparrow$0.45)}} & 52.72\textsubscript{\textcolor{blue}{($\uparrow$0.30)}} & 93.43\textsubscript{\textcolor{blue}{($\uparrow$0.38)}} & 77.42\textsubscript{\textcolor{blue}{($\uparrow$0.51)}} & 74.17\textsubscript{\textcolor{blue}{($\uparrow$0.45)}} & 95.13\textsubscript{\textcolor{red}{($\downarrow$0.04)}} & 88.90\textsubscript{\textcolor{blue}{($\uparrow$0.32)}} & 67.81\textsubscript{\textcolor{blue}{($\uparrow$0.13)}} & 30.42\textsubscript{\textcolor{blue}{($\uparrow$0.39)}} & 55.01\textsubscript{\textcolor{red}{($\downarrow$0.07)}} & 71.17\textsubscript{\textcolor{blue}{($\uparrow$0.28)}} \\
\rowcolor{blue!15}\textbf{\name} (Ours) & 76.57\textsubscript{\textcolor{blue}{($\uparrow$0.37)}} & 54.14\textsubscript{\textcolor{blue}{($\uparrow$1.71)}} & 93.87\textsubscript{\textcolor{blue}{($\uparrow$0.82)}} & 78.31\textsubscript{\textcolor{blue}{($\uparrow$1.41)}} & 74.83\textsubscript{\textcolor{blue}{($\uparrow$1.11)}} & 95.54\textsubscript{\textcolor{blue}{($\uparrow$0.37)}} & 89.34\textsubscript{\textcolor{blue}{($\uparrow$0.77)}} & 68.72\textsubscript{\textcolor{blue}{($\uparrow$1.04)}} & 33.12\textsubscript{\textcolor{blue}{($\uparrow$3.09)}} & 53.74\textsubscript{\textcolor{red}{($\downarrow$1.35)}} & 71.82\textsubscript{\textcolor{blue}{($\uparrow$0.93)}} \\
\rowcolor{blue!10}\textbf{\name} + Ensemble (Ours) & 75.92\textsubscript{\textcolor{red}{($\downarrow$0.28)}} & 55.08\textsubscript{\textcolor{blue}{($\uparrow$2.66)}} & 93.08\textsubscript{\textcolor{blue}{($\uparrow$0.03)}} & 79.38\textsubscript{\textcolor{blue}{($\uparrow$2.47)}} & 76.79\textsubscript{\textcolor{blue}{($\uparrow$3.07)}} & 95.94\textsubscript{\textcolor{blue}{($\uparrow$0.77)}} & 89.79\textsubscript{\textcolor{blue}{($\uparrow$1.21)}} & 71.13\textsubscript{\textcolor{blue}{($\uparrow$3.45)}} & 35.34\textsubscript{\textcolor{blue}{($\uparrow$5.32)}} & 52.19\textsubscript{\textcolor{red}{($\downarrow$2.90)}} & 72.46\textsubscript{\textcolor{blue}{($\uparrow$1.58)}} \\
\bottomrule
\end{tabular}
\end{adjustbox}
\end{table*}

\subsection{Error analysis}
\cref{tab:imagenets_error} and \cref{tab:fg_error} present the standard deviation of three random runs with different seeds for zero-shot image classification on the OOD and fine-grained benchmarks, respectively.
The randomness of \namemem\ mainly stems from random data augmentation and one-step optimization, similar to TPT.
Additionally, \namemae\ introduces an additional source of randomness through its masking strategy.
Nevertheless, our method achieves an error magnitude comparable to that of TPT.

\subsection{Expected Calibration Error}
\cref{tab:imagenets_calib} presents the calibration results on the OOD benchmark, while \cref{tab:fg_calib} shows the results on the fine-grained benchmark for each dataset.
The comparison includes our method, TPT \cite{shu2022test}, and C-TPT \cite{yoon2024c}.
The results show that \namemae\ (\ie, MAE loss) achieves calibration performance comparable to or surpassing that of C-TPT across a wide range of categories, highlighting the effective calibration properties of MAE loss.

\subsection{Scalability Analysis of Our Method}
In this section, we evaluate the scalability of our proposed method by applying it to a larger baseline model.
\cref{tab:imagenets_vit_l} and \cref{tab:fg_vit_l} show the results obtained using the pretrained CLIP-ViT-L/14 on the OOD and fine-grained benchmarks, respectively.
LoRA is applied exclusively to the transformer architecture in layers 23 and 24 of the image encoder, targeting the key, query, value, and output matrices with a rank of 16, and the LoRA scale $\gamma$ is set to 2.
All other experimental parameters are consistent with those in the main paper. 
The results demonstrate that \name\ consistently outperforms the baseline CLIP-ViT-L/14 across both benchmarks and multiple categories while maintaining the zero-shot setting.
It also demonstrates performance improvements when combined with the ensemble text prompts, exhibiting generalization properties to text prompts similar to those observed with CLIP-ViT-B/16.
Performance improvements are observed with both types of loss (\ie, \namemem\ and \namemae), highlighting the robustness of our method and its scalability to larger baseline models.

\section{Qualitative Analysis}
\cref{tab:tsne} shows the t-SNE visualization of image features after the image encoder for various evaluation datasets, comparing the baseline CLIP-ViT-B/16 and our method.
The results show that our approach achieves better class separation than the baseline, indicating improved classification performance on the test data.
Additionally, the visualizations highlight that the type of test loss affects how class separation is achieved.

\begin{table*}[t]
\centering
\caption{\textbf{t-SNE visualizations.} The plot colors indicate the category classes of each dataset.}
\label{tab:tsne}
\begin{adjustbox}{width=\textwidth}
% Define a custom column type for vertical centering
\newcolumntype{M}[1]{>{\centering\arraybackslash}m{#1}}

\begin{tabular}{M{1cm}M{3.8cm}M{3.8cm}M{3.8cm}M{3.8cm}} % First column for row labels
    & CLIP-ViT-B/16 & \namemem & \namemae & \name \\
    ImageNet-A & 
    \includegraphics[width=0.23\textwidth]{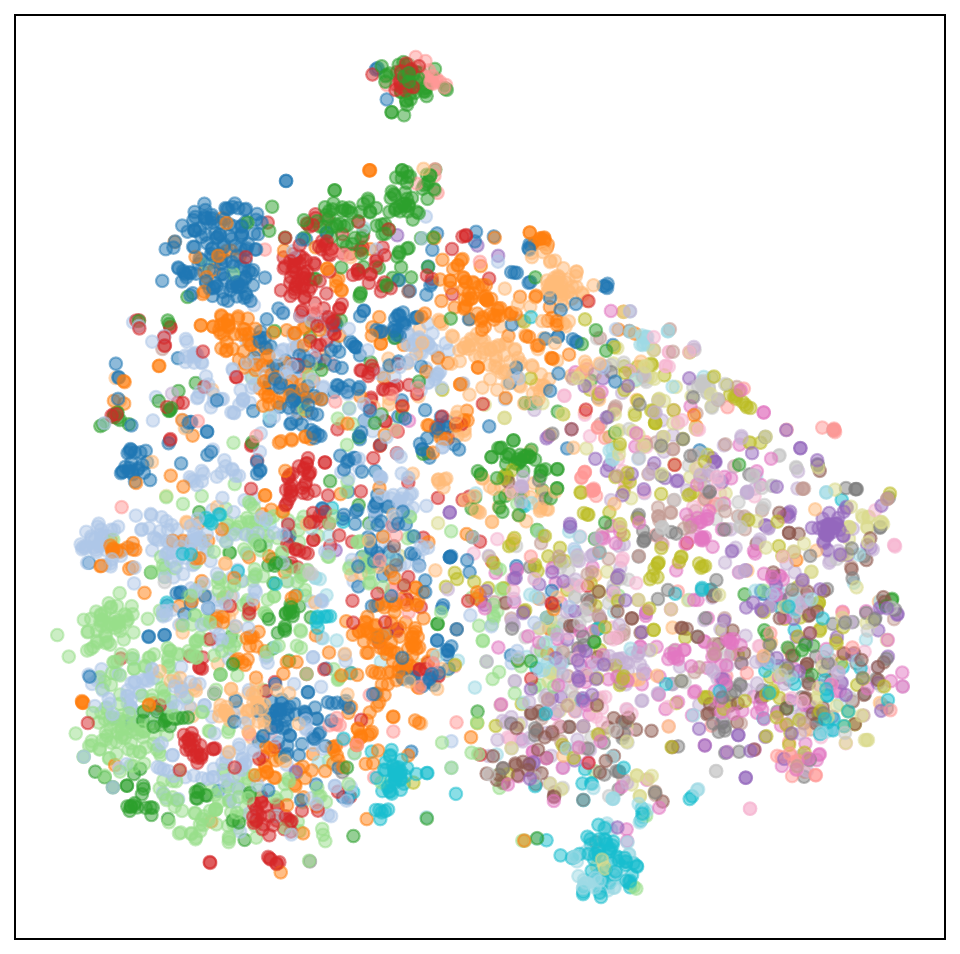} & 
    \includegraphics[width=0.23\textwidth]{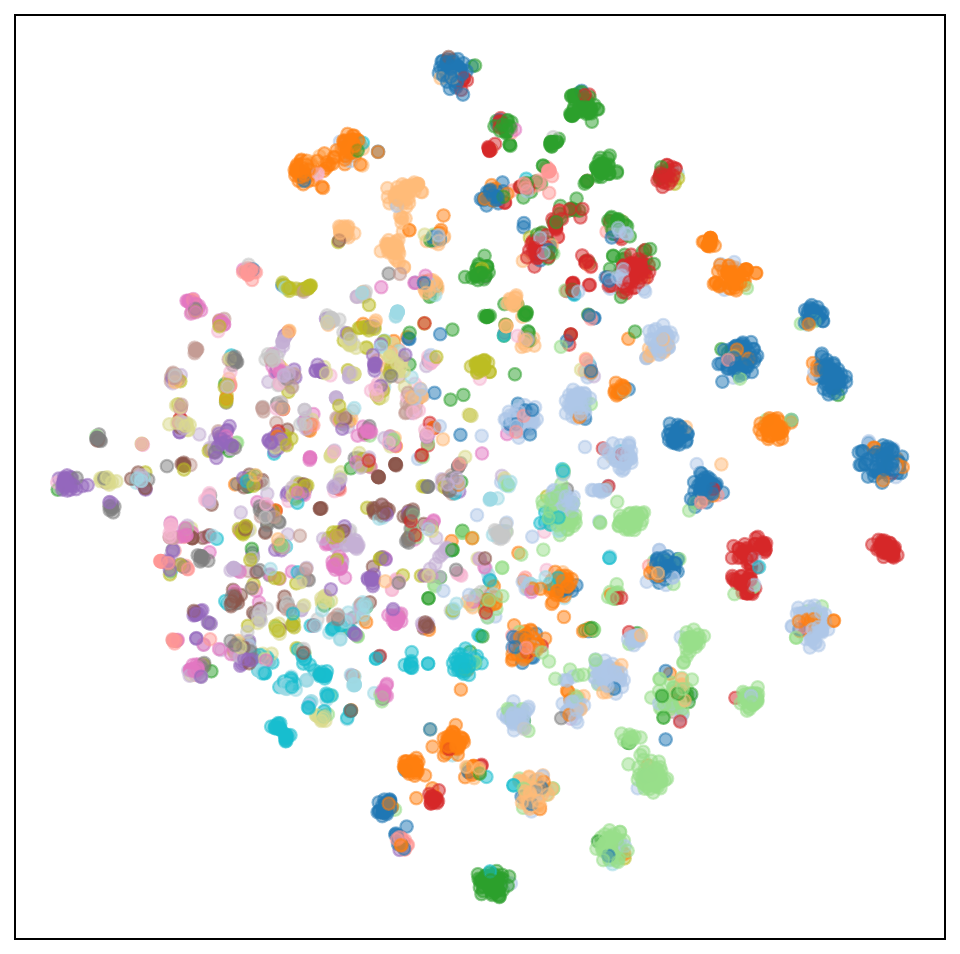} & 
    \includegraphics[width=0.23\textwidth]{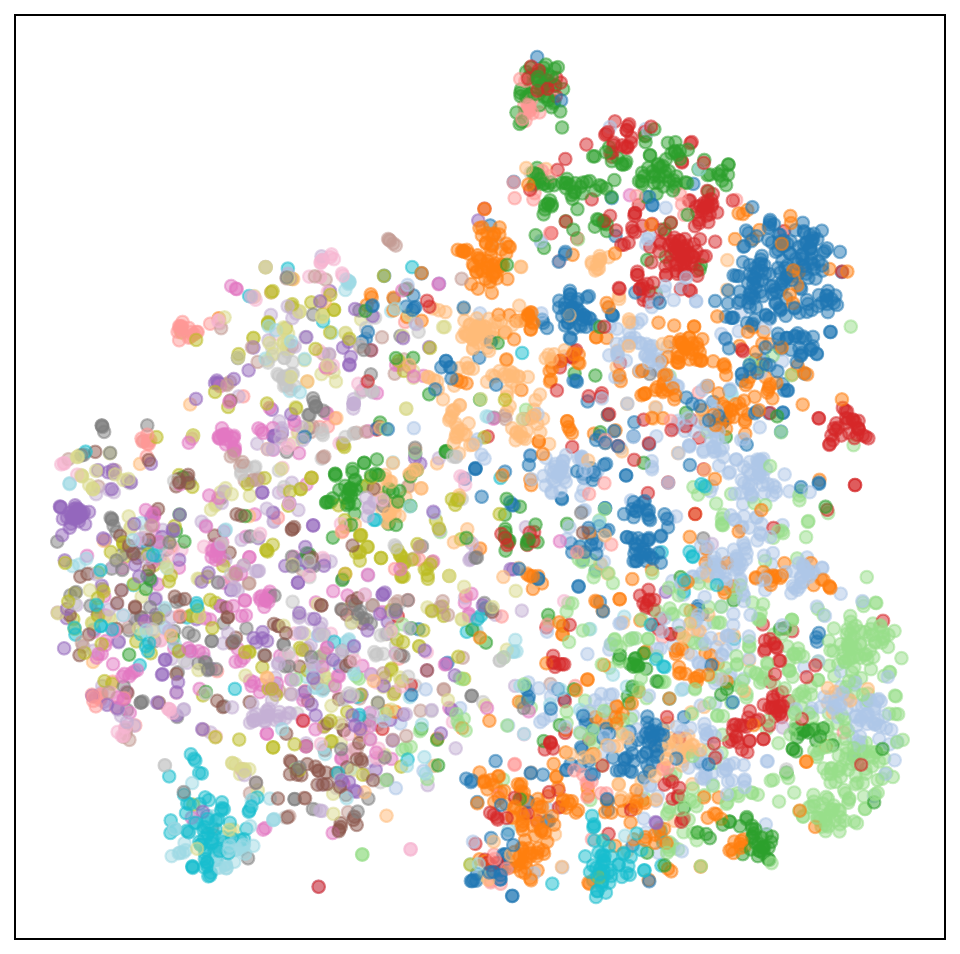} & 
    \includegraphics[width=0.23\textwidth]{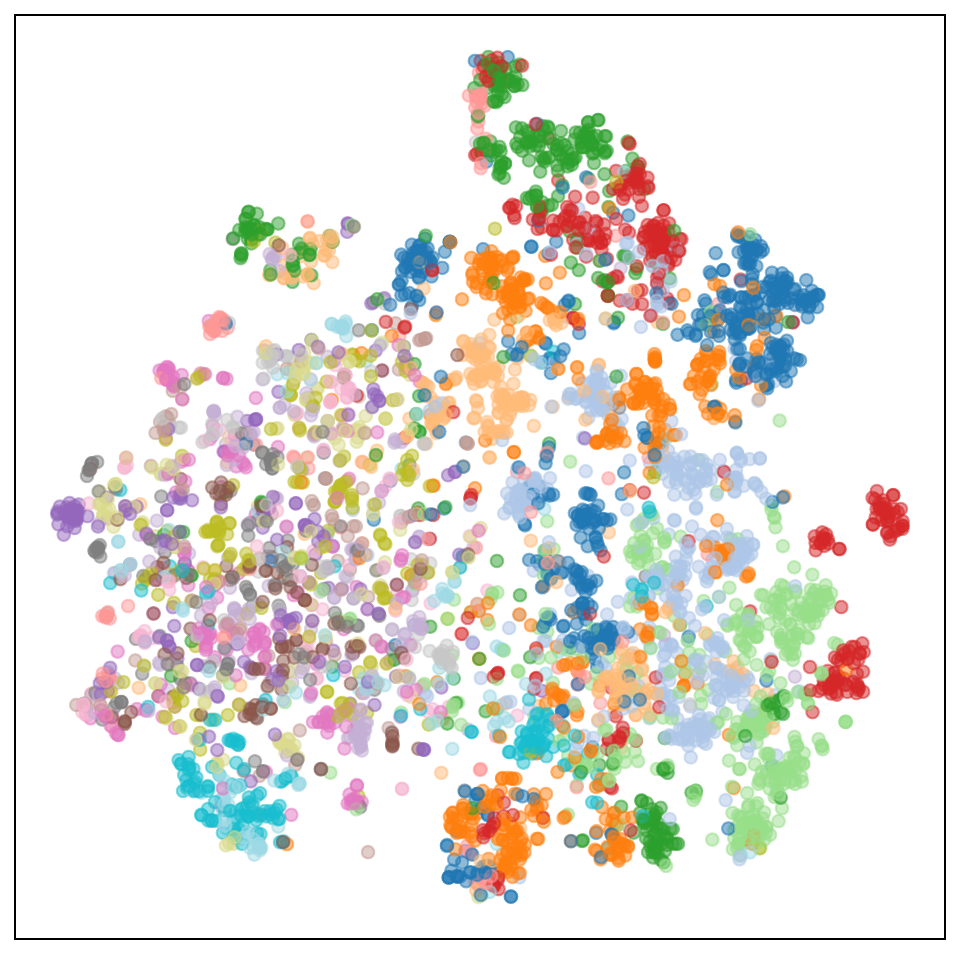} \\
    
    DTD & 
    \includegraphics[width=0.23\textwidth]{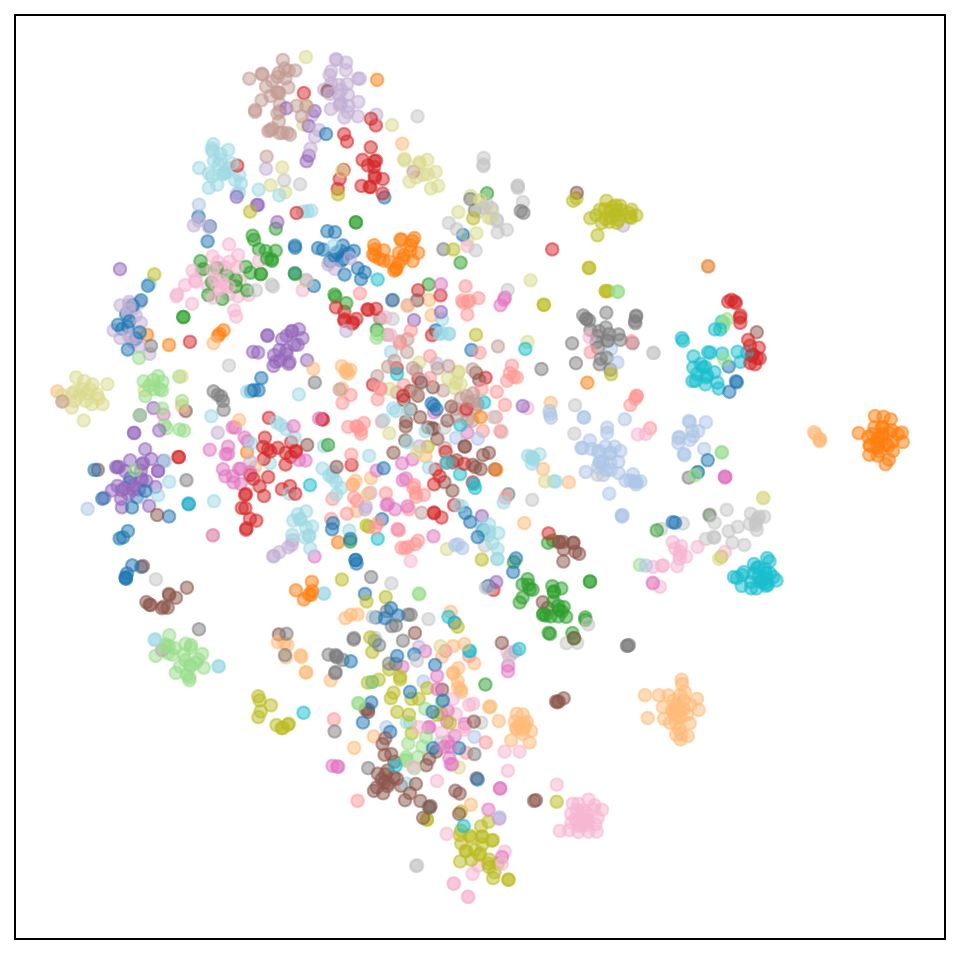} & 
    \includegraphics[width=0.23\textwidth]{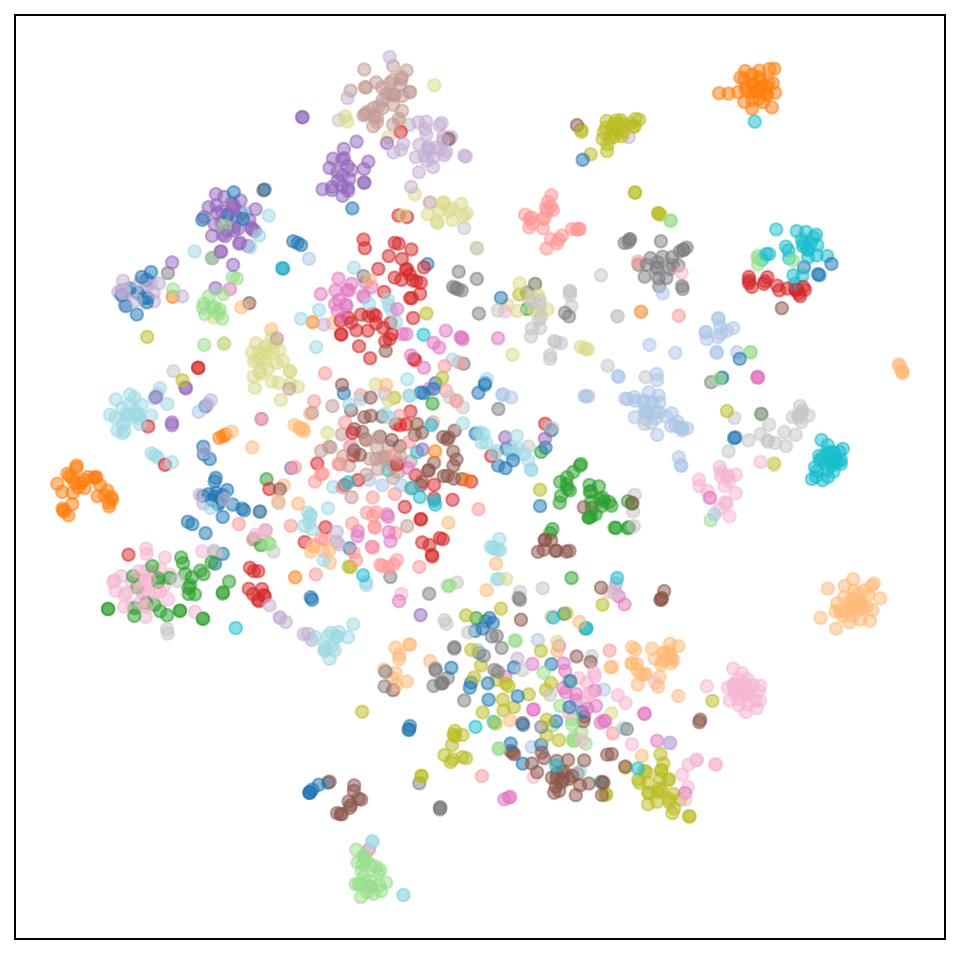} & 
    \includegraphics[width=0.23\textwidth]{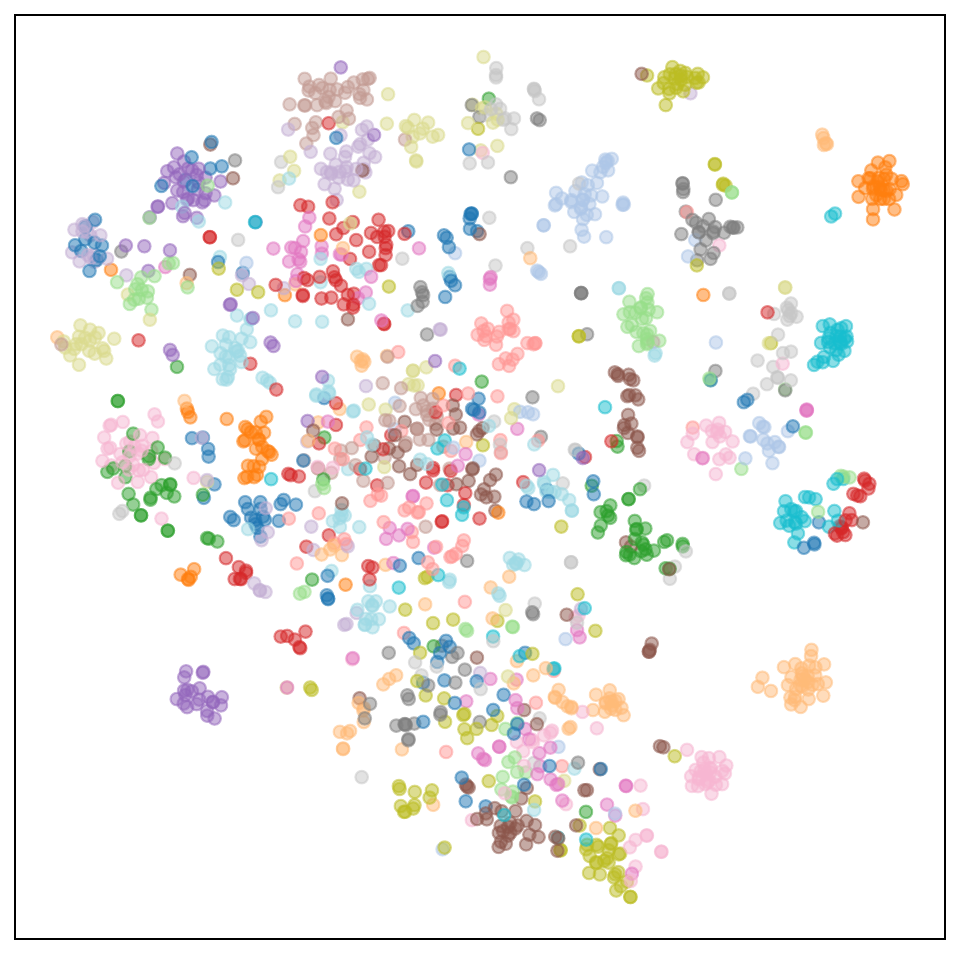} & 
    \includegraphics[width=0.23\textwidth]{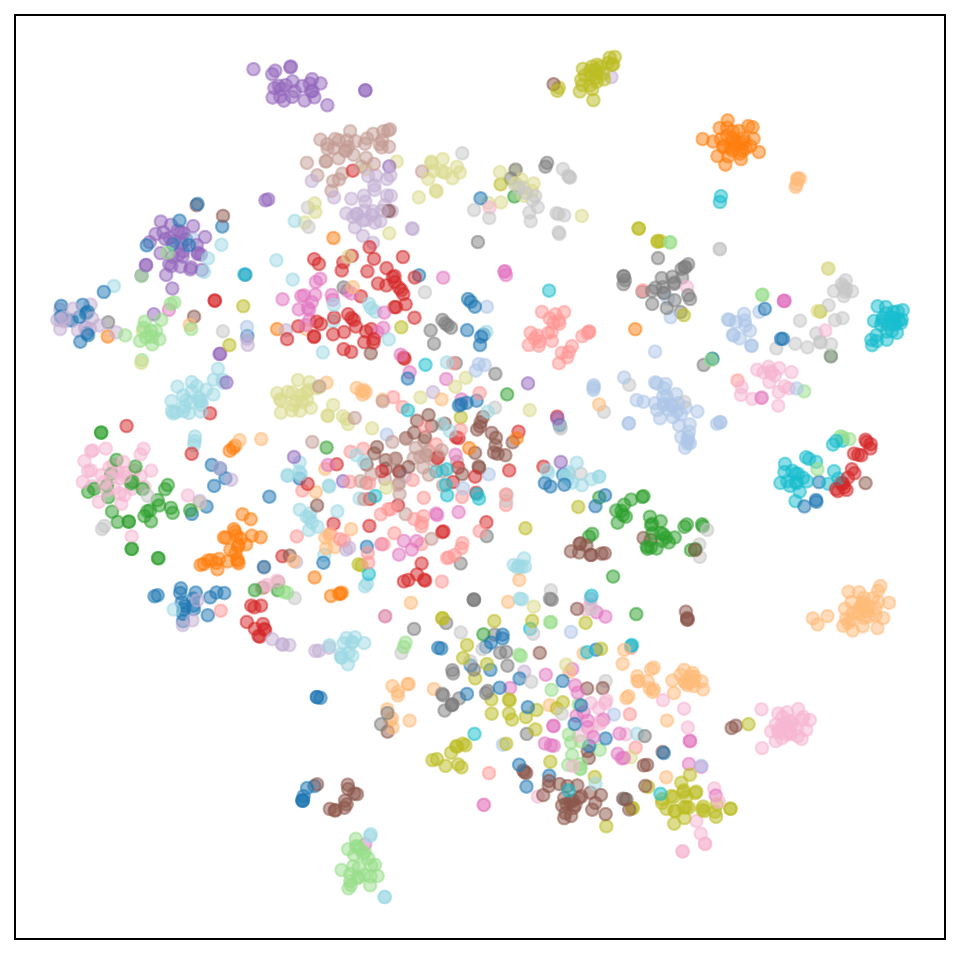} \\

    Food101 & 
    \includegraphics[width=0.23\textwidth]{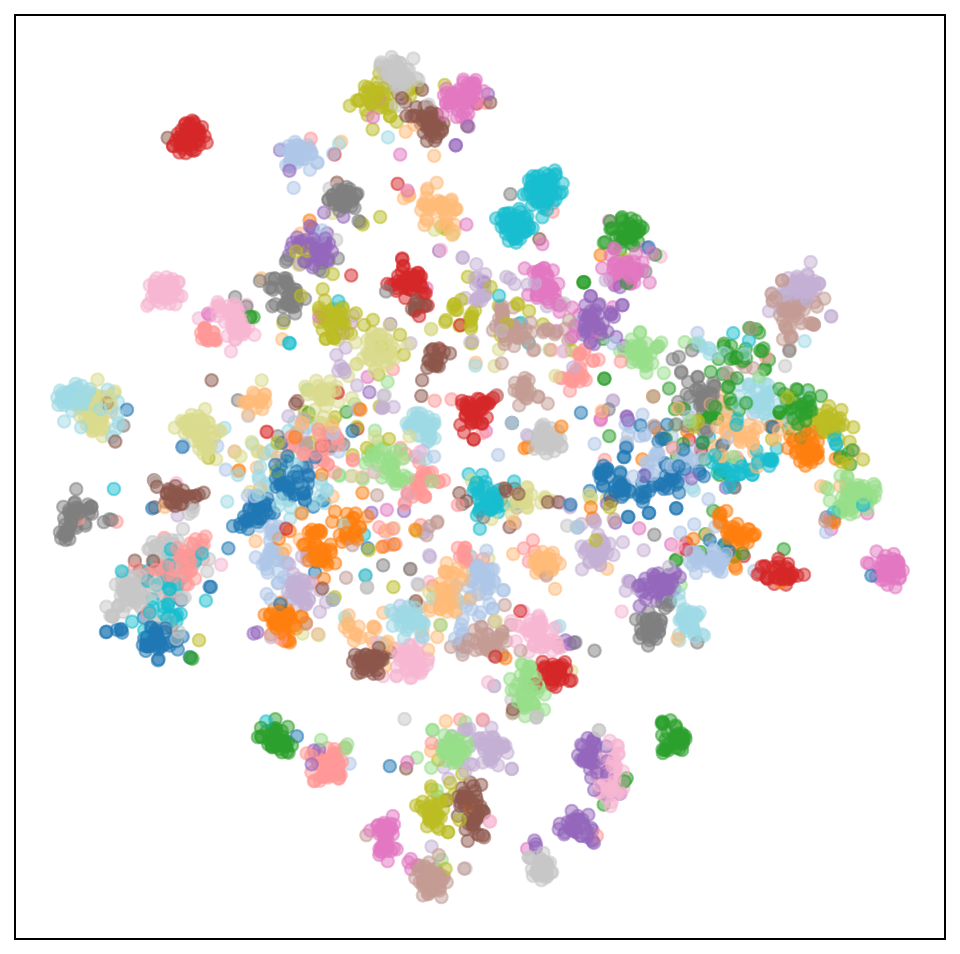} & 
    \includegraphics[width=0.23\textwidth]{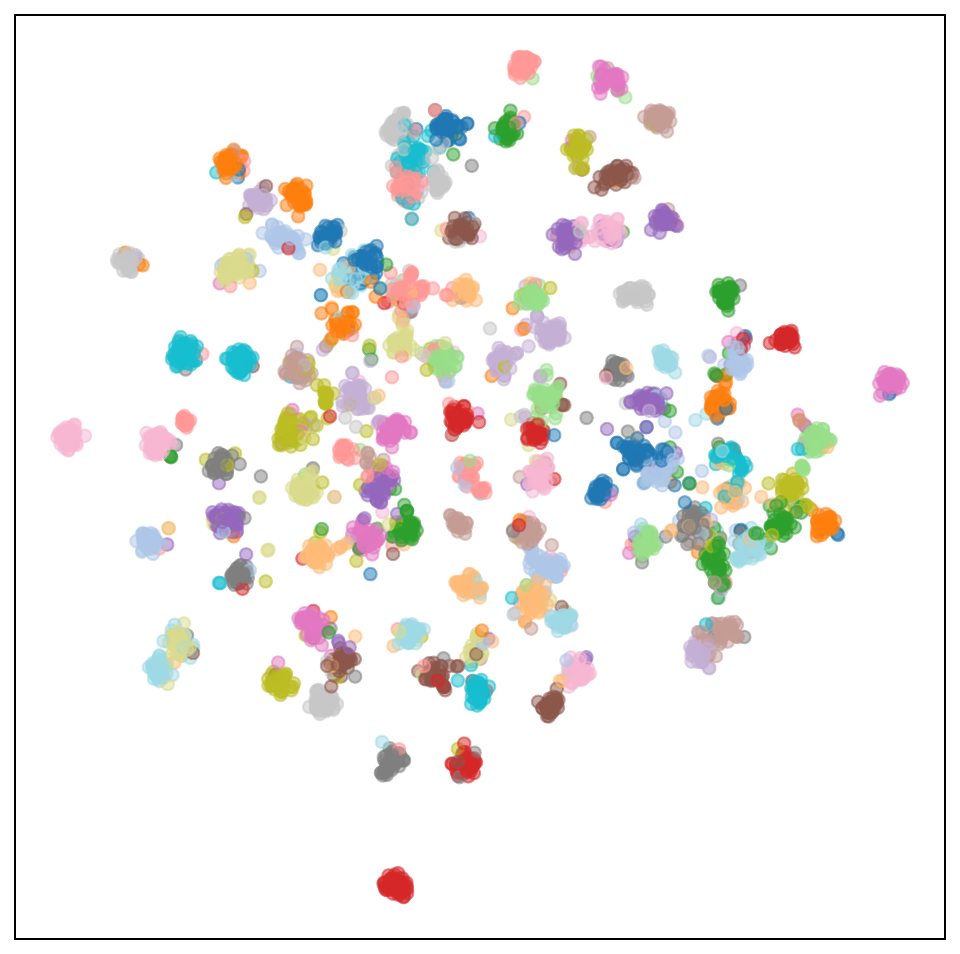} & 
    \includegraphics[width=0.23\textwidth]{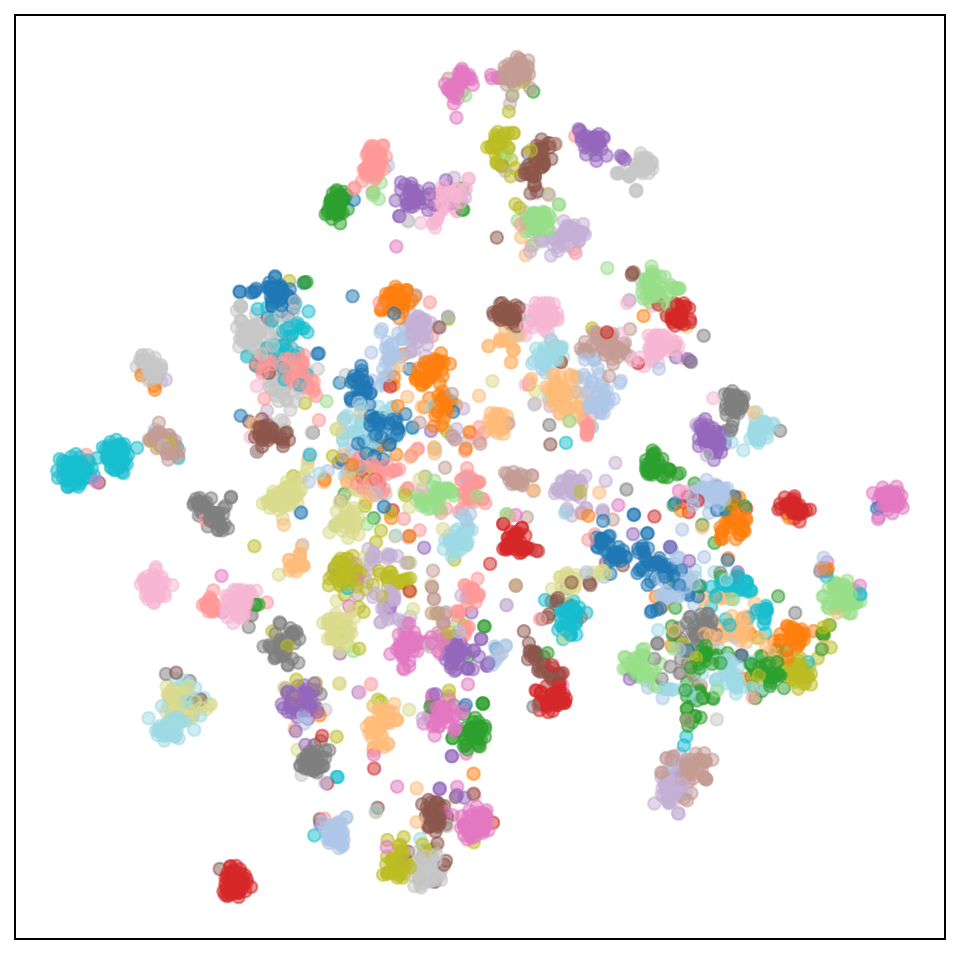} & 
    \includegraphics[width=0.23\textwidth]{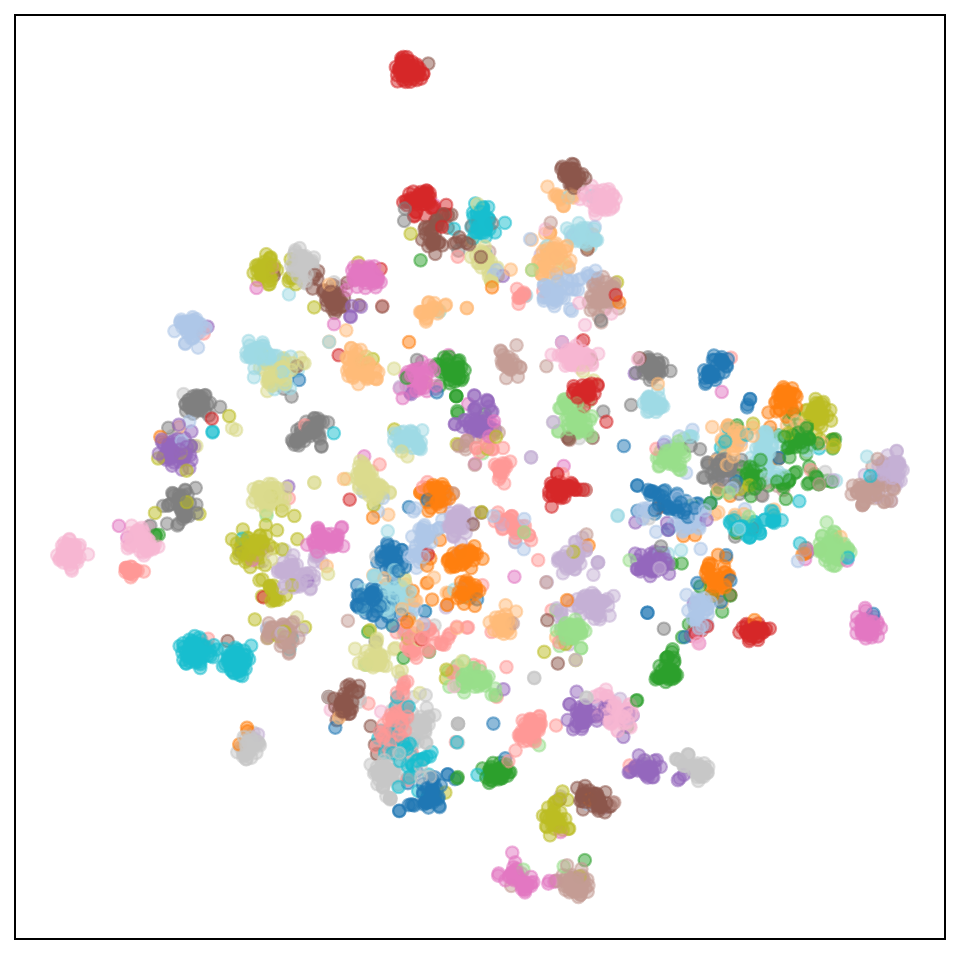} \\

    UCF101 & 
    \includegraphics[width=0.23\textwidth]{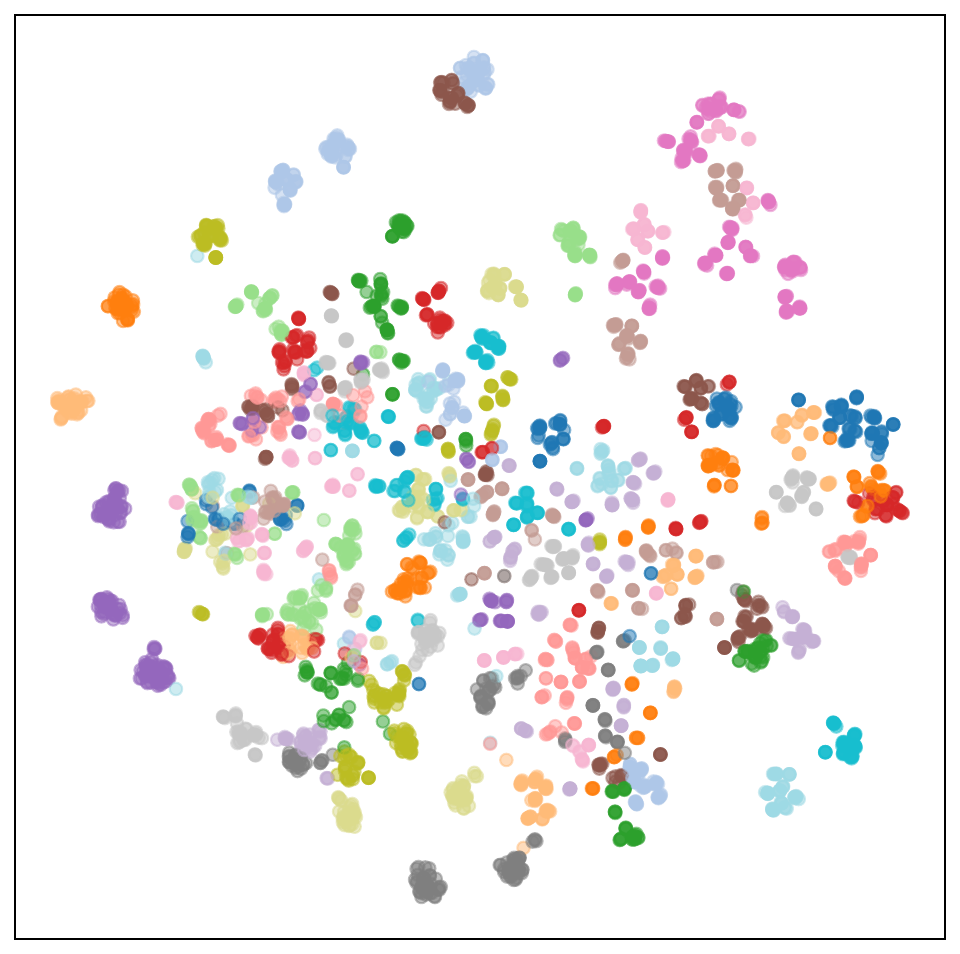} & 
    \includegraphics[width=0.23\textwidth]{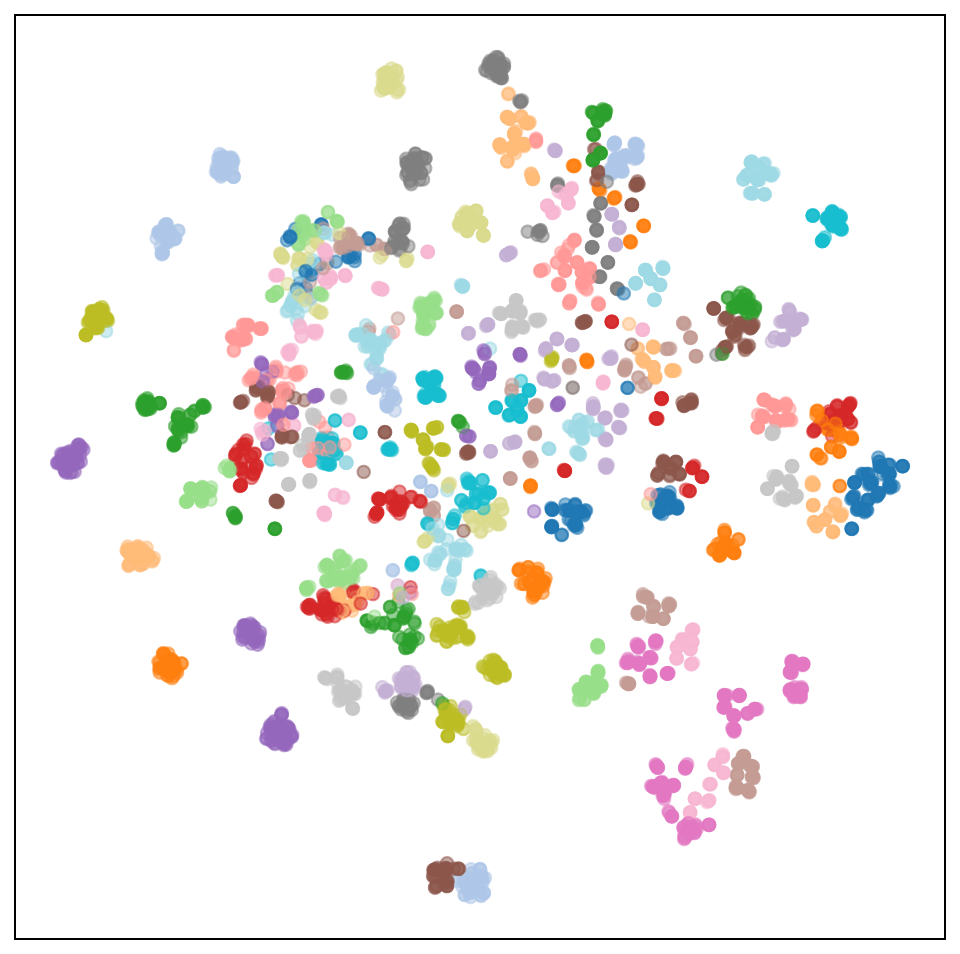} & 
    \includegraphics[width=0.23\textwidth]{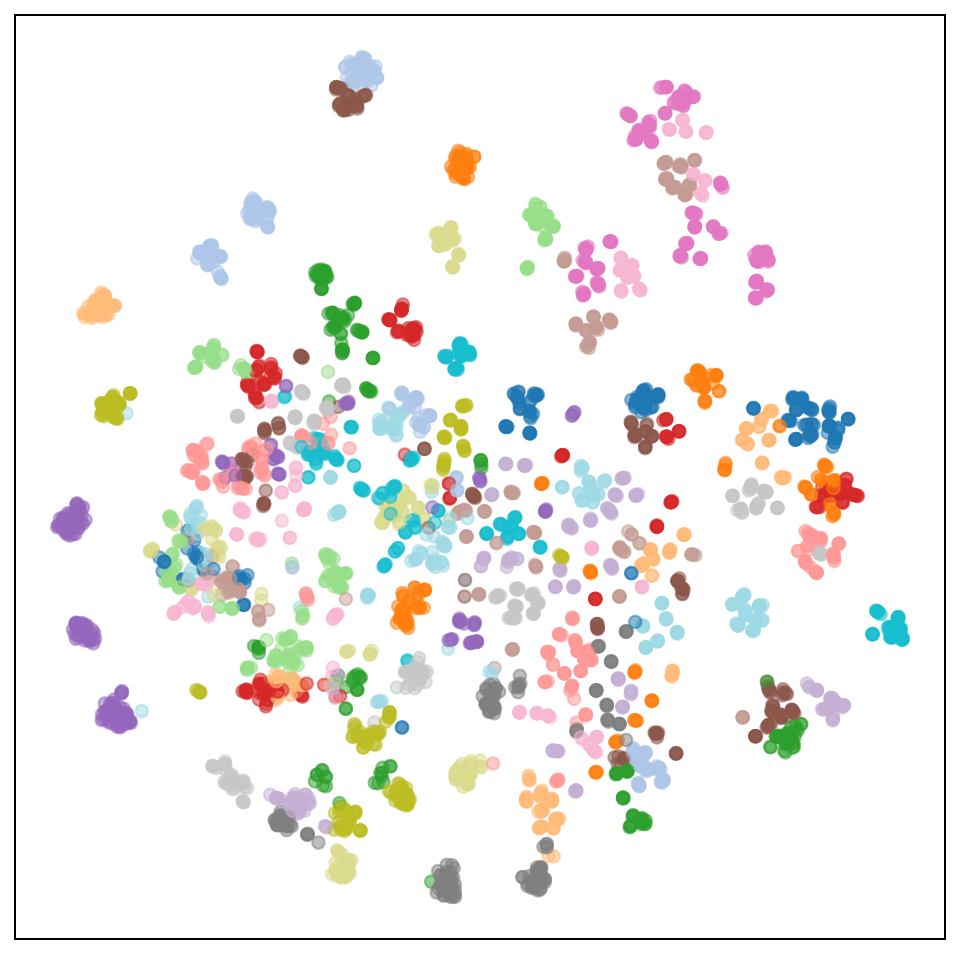} & 
    \includegraphics[width=0.23\textwidth]{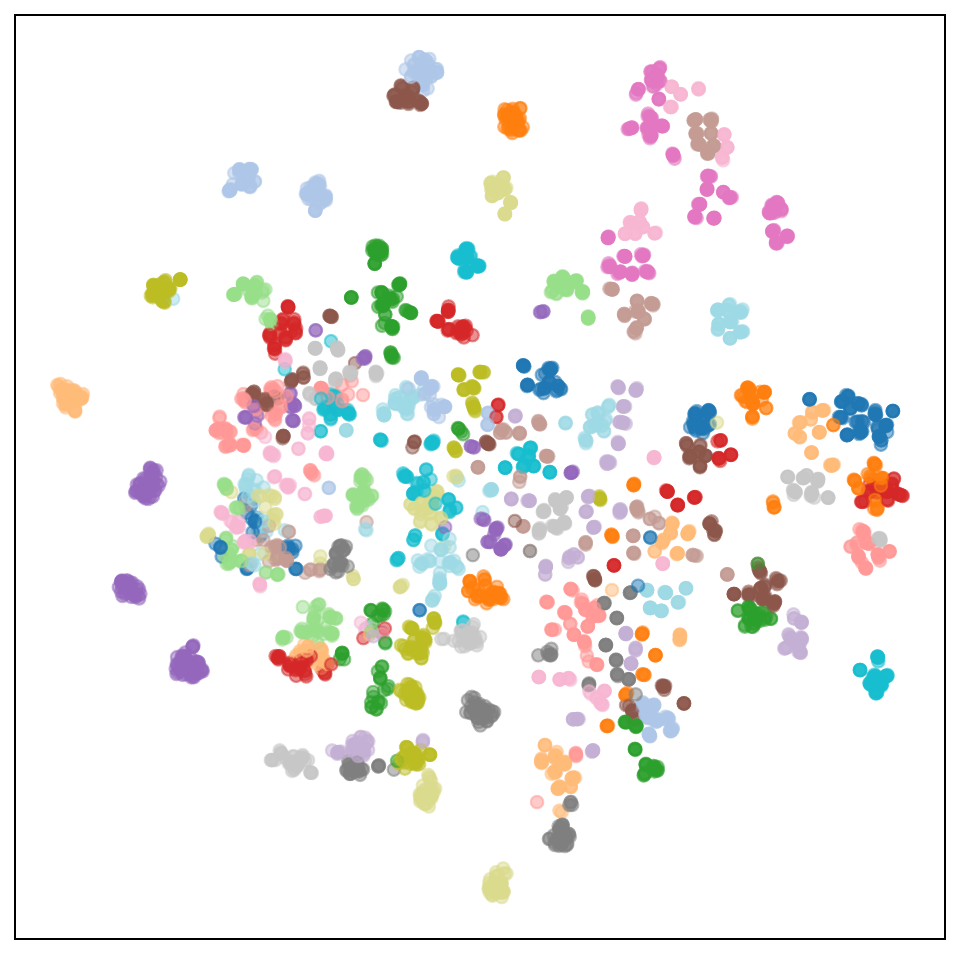} \\
    
    EuroSAT & 
    \includegraphics[width=0.23\textwidth]{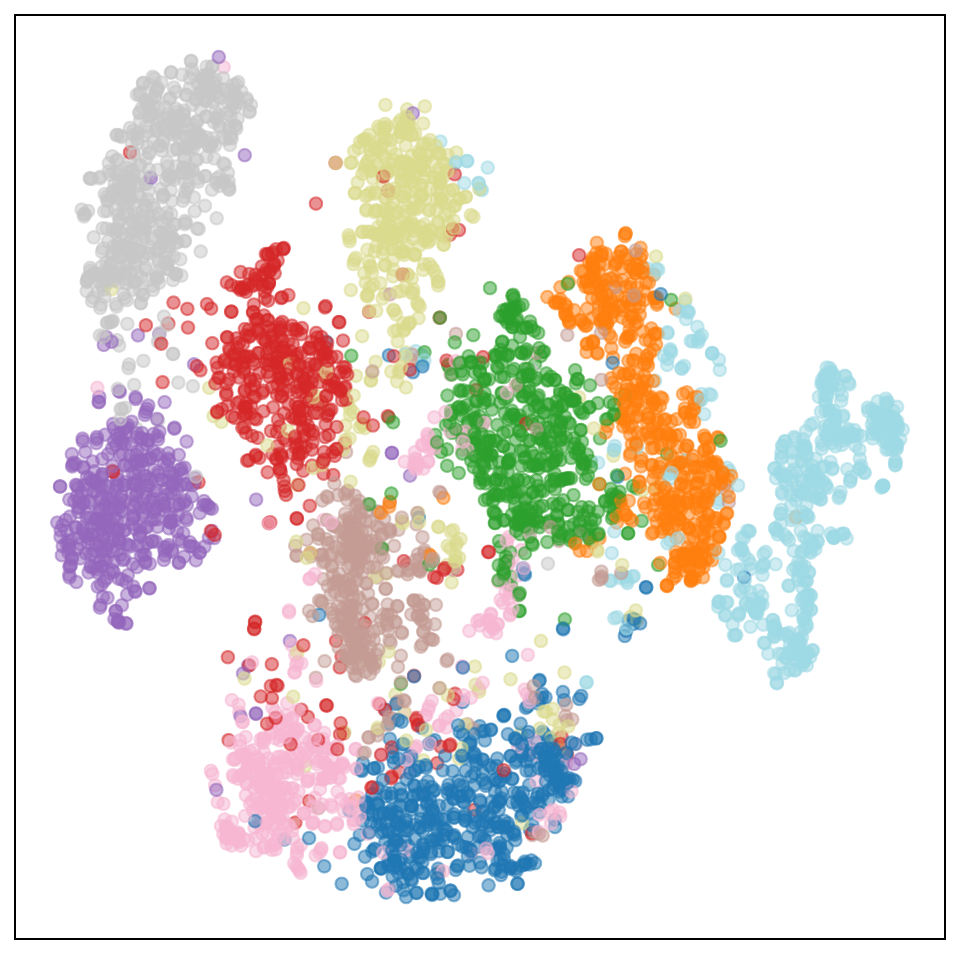} & 
    \includegraphics[width=0.23\textwidth]{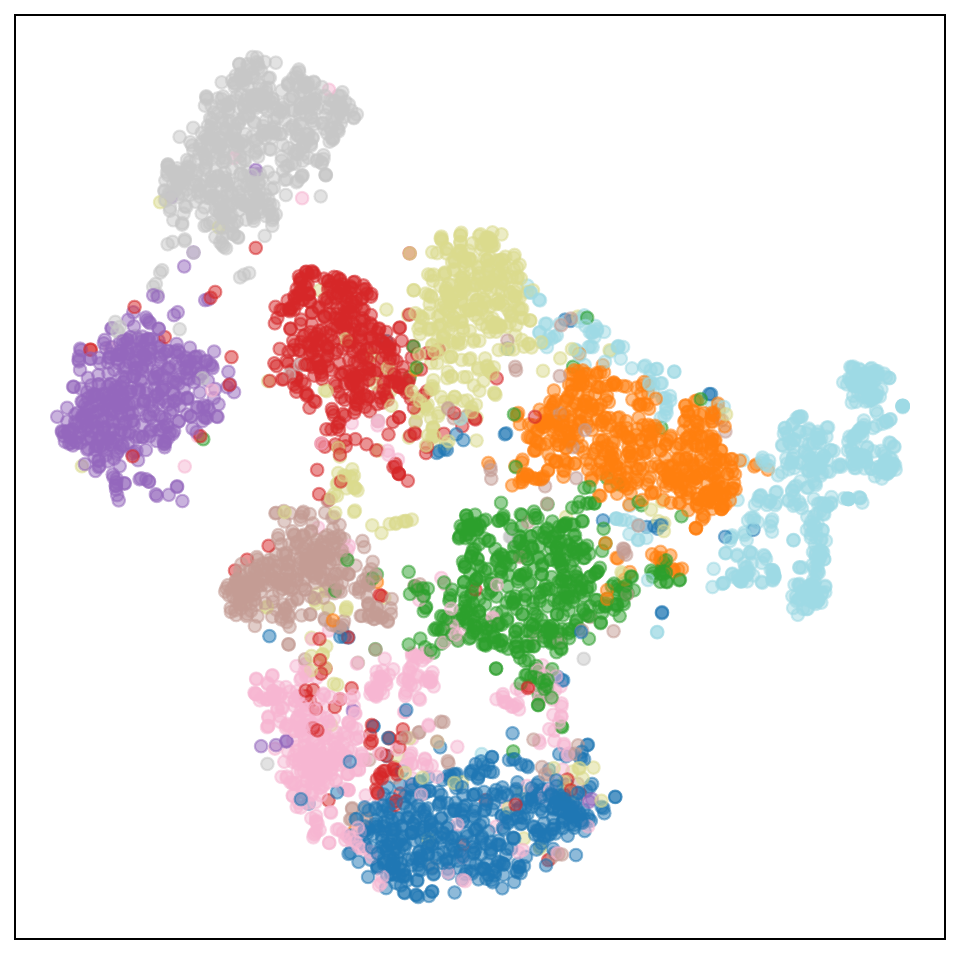} & 
    \includegraphics[width=0.23\textwidth]{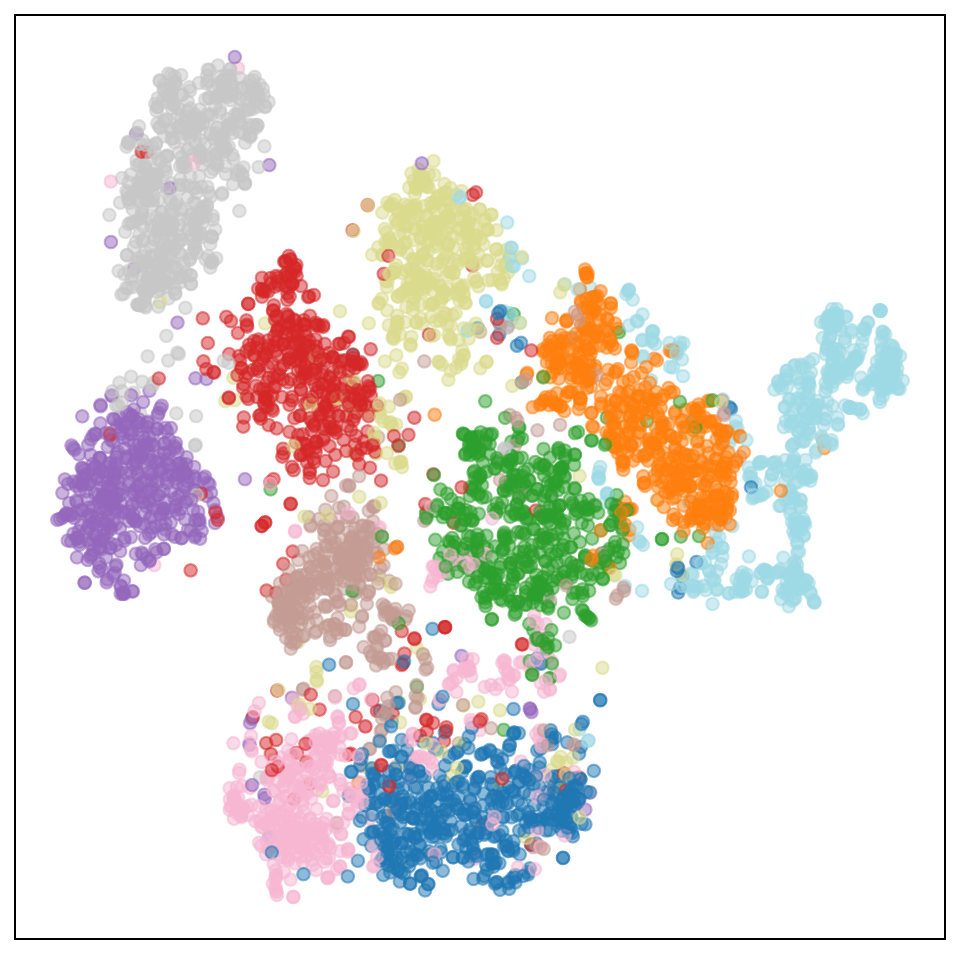} & 
    \includegraphics[width=0.23\textwidth]{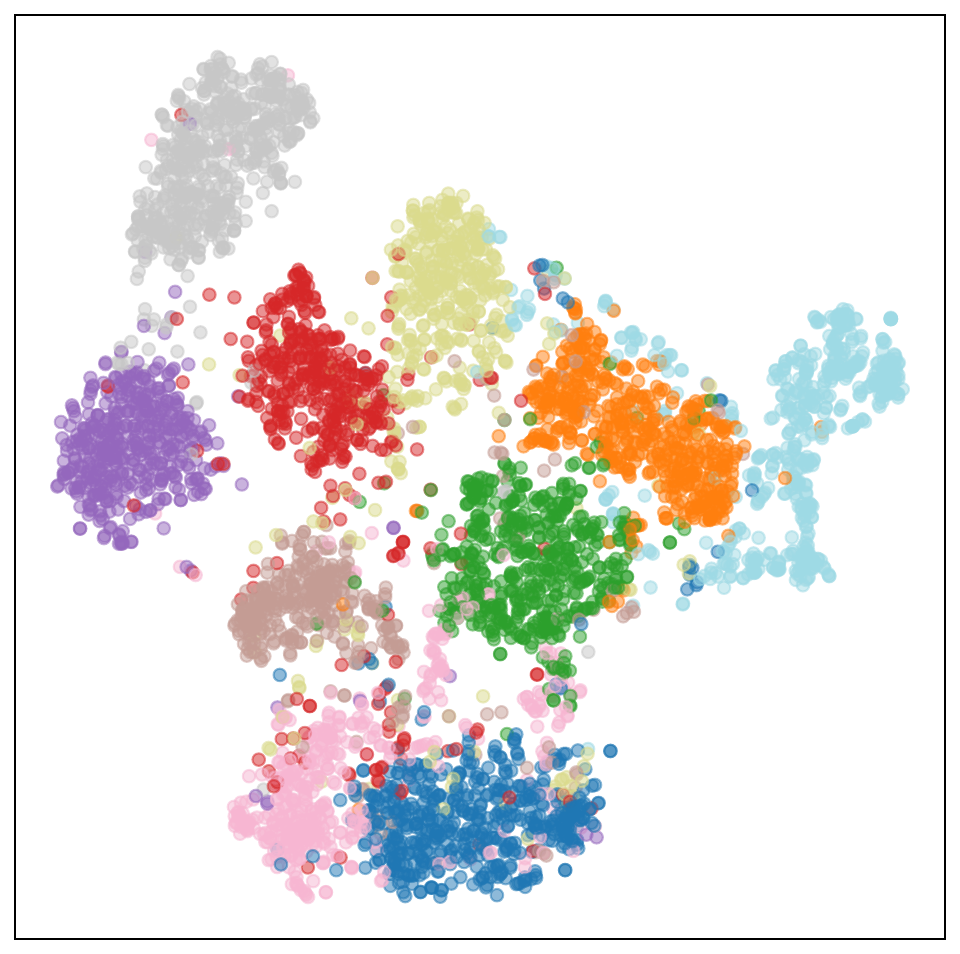} \\
\end{tabular}
\end{adjustbox}
\end{table*}
